# Supplementary material for: Momentum-resolved time evolution with matrix product states
Source: arXiv:2201.07314 source file (2022-06-07)

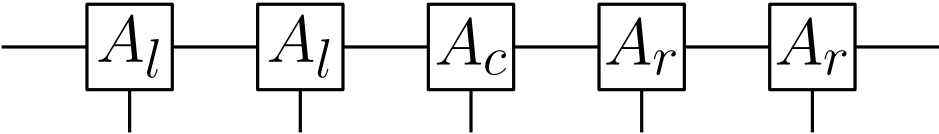

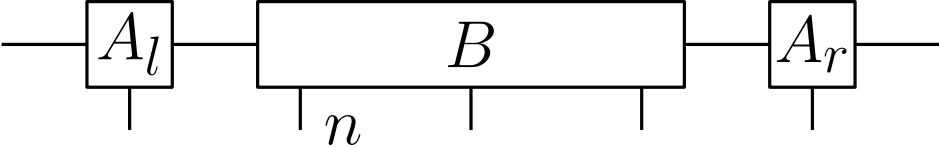

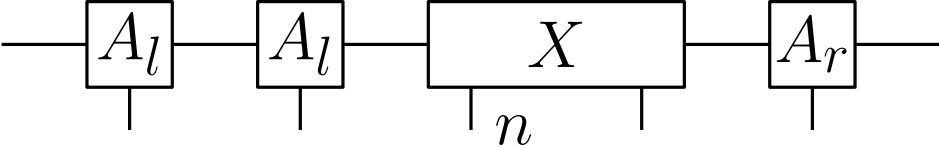

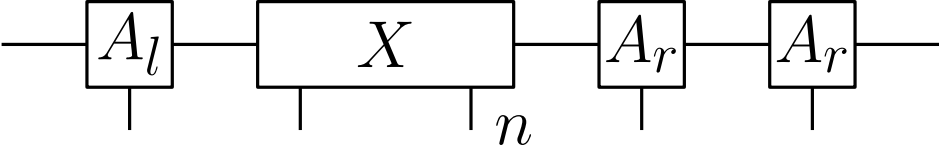

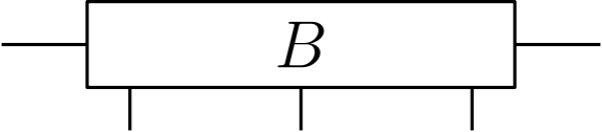

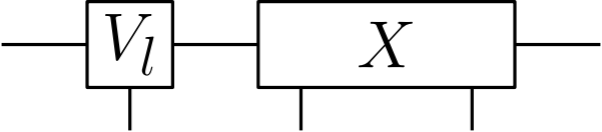

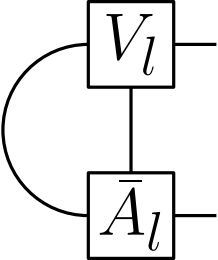

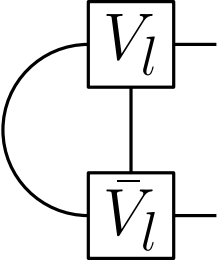

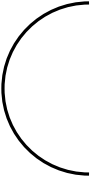

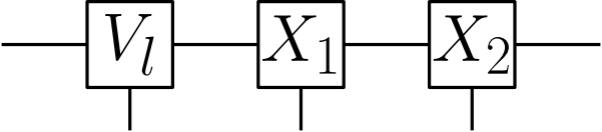

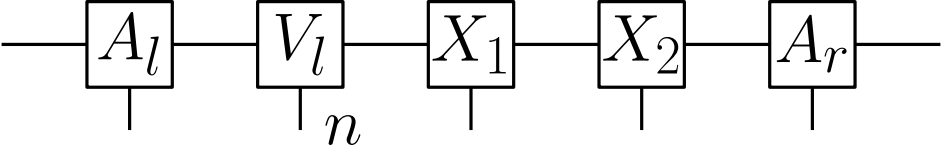

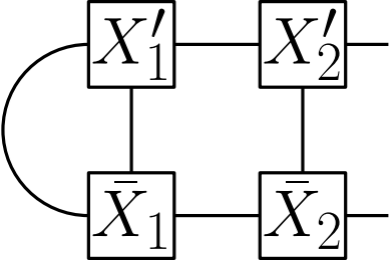

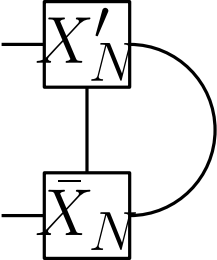

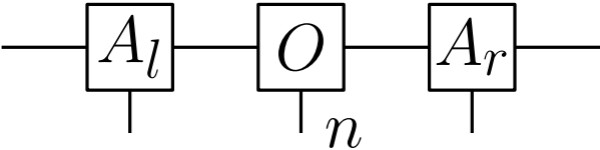

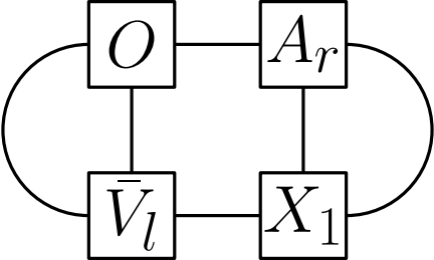

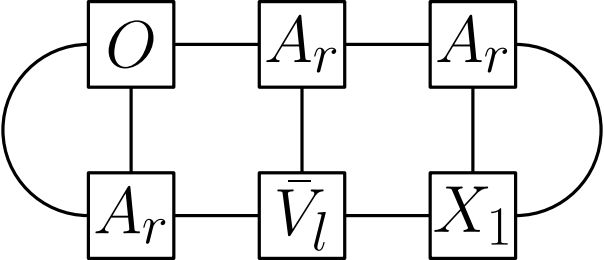

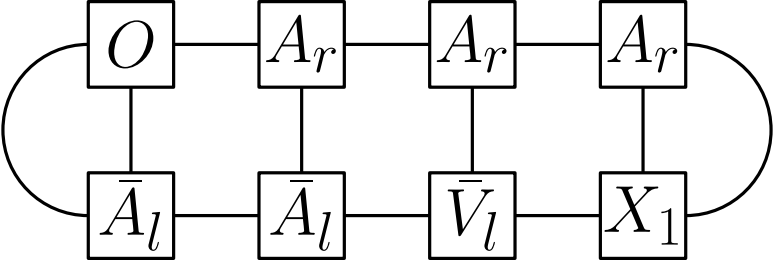

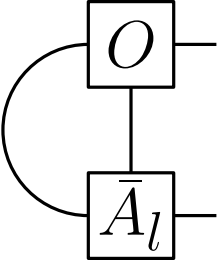

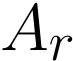

$A_r$

$\overline{A_l}$

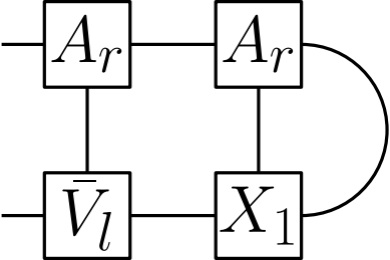

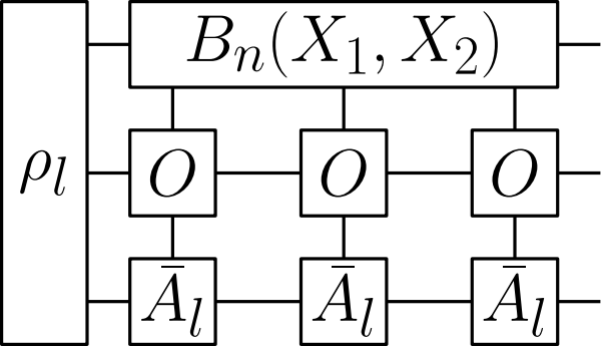

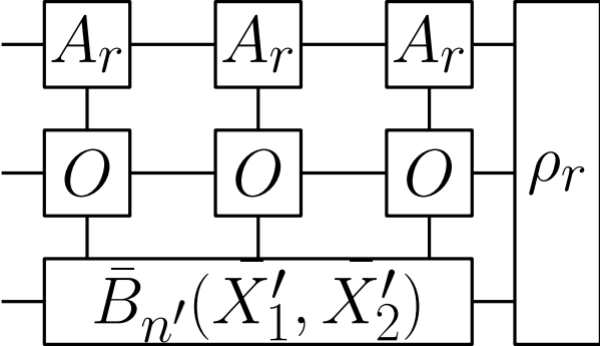

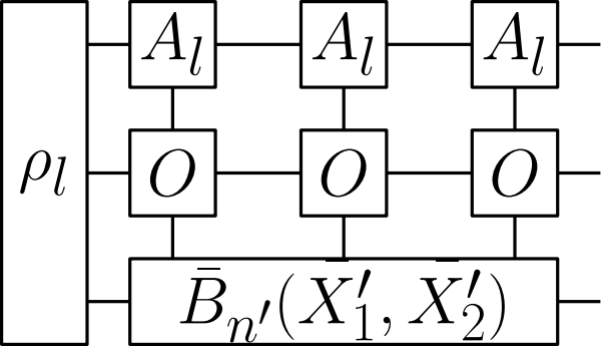

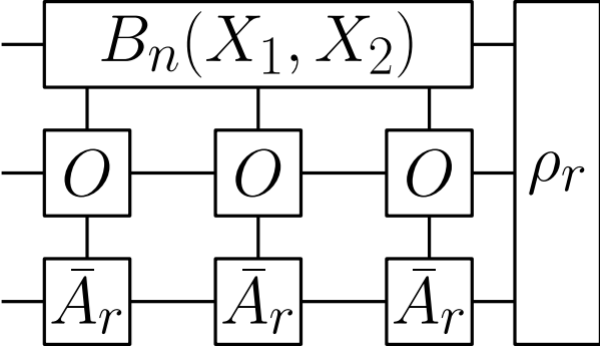

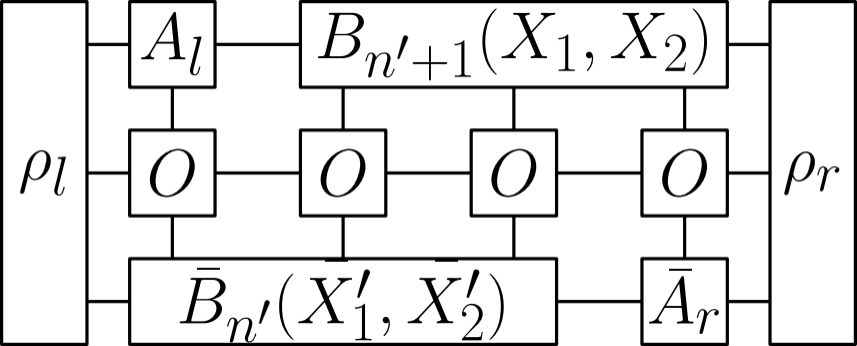

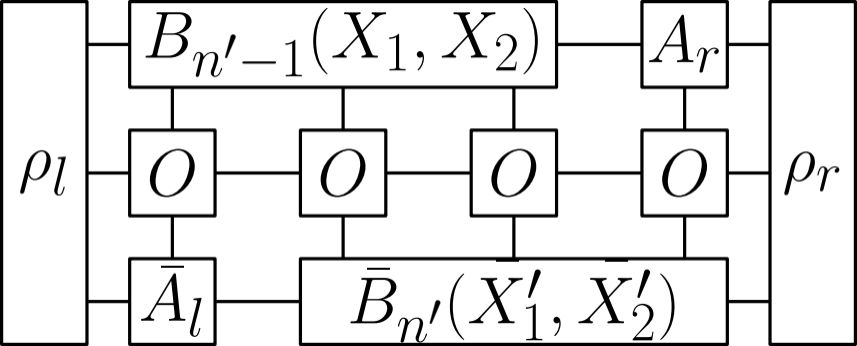

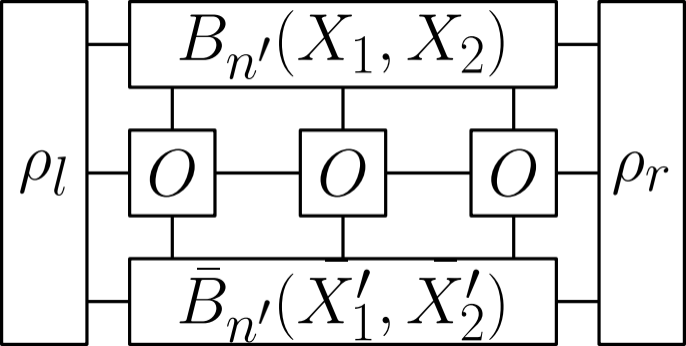

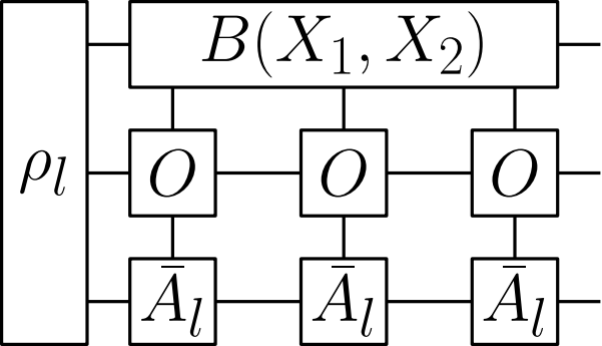

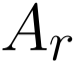

A diagram showing three square boxes stacked vertically. Each box has a horizontal line passing through its center. The top box contains the label  $A_r$ , the middle box contains the label  $O$ , and the bottom box contains the label  $A_l$ . The boxes are connected by vertical lines, and each box has a horizontal line extending from its left and right sides.

$$A_r$$
$$O$$
$$\bar{A}_l$$

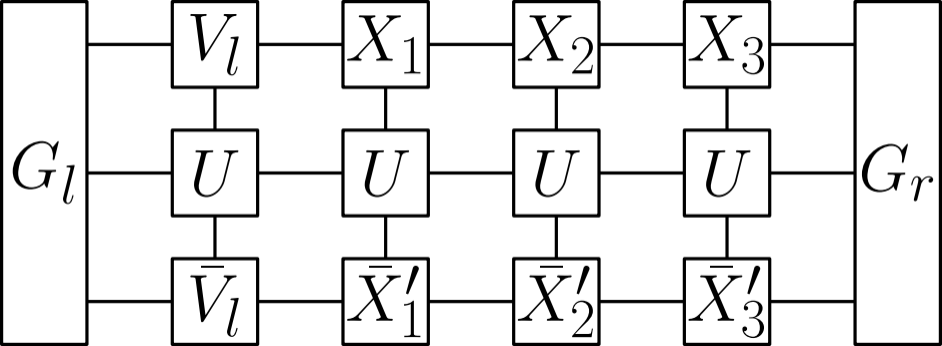

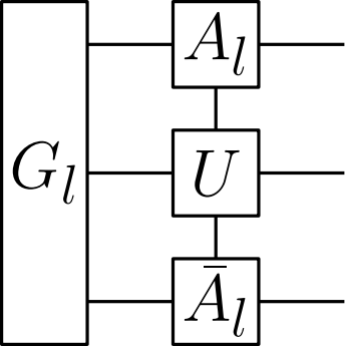

$G_l$

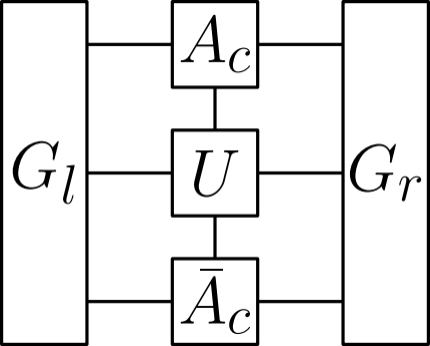

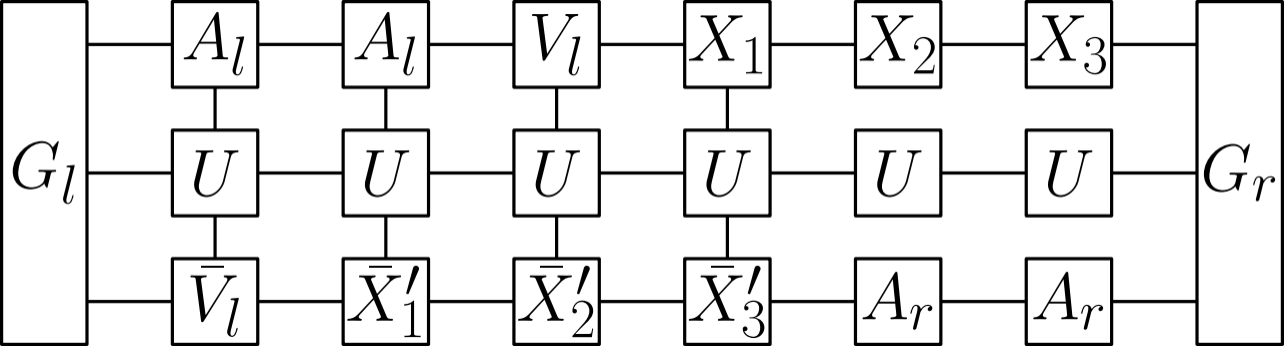

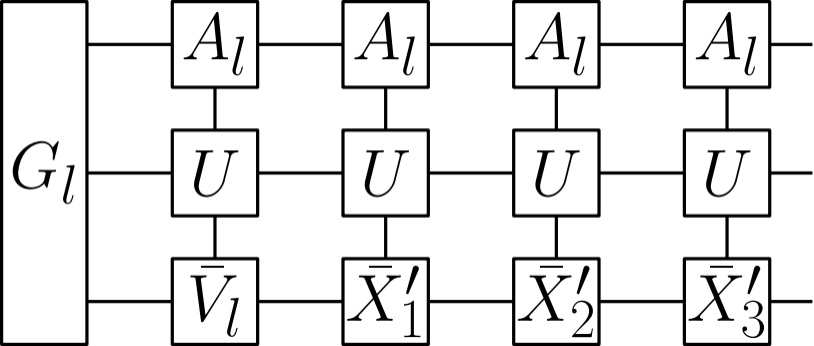

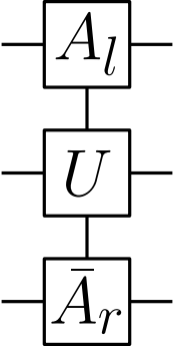

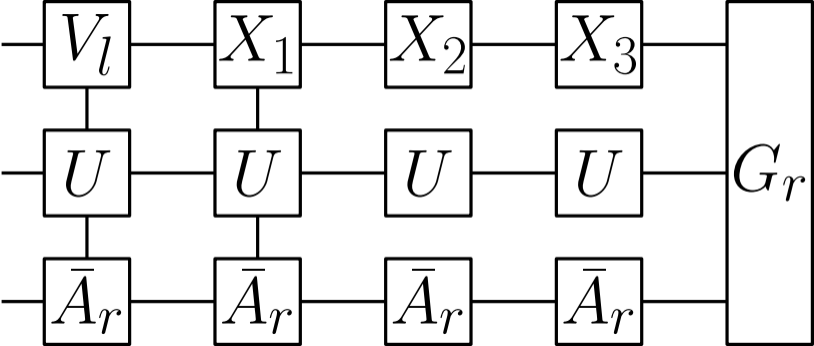

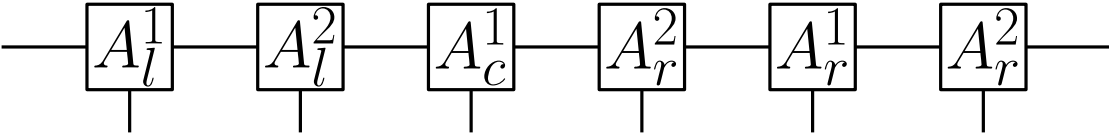

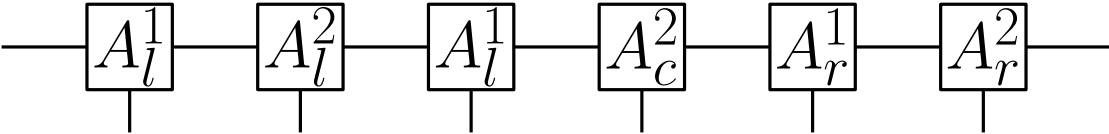

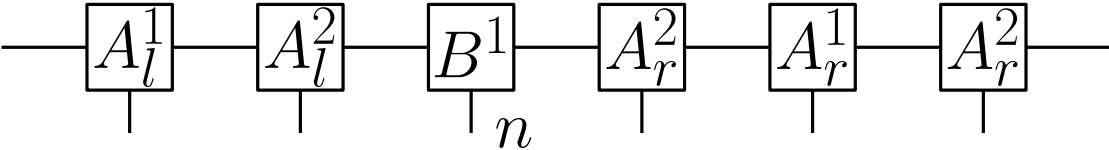

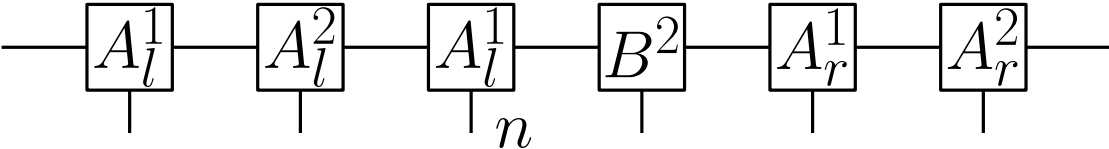

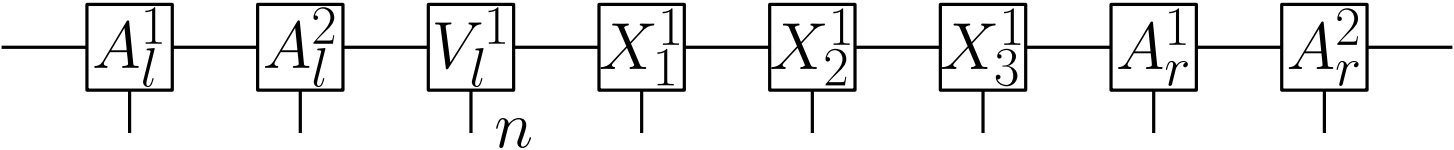

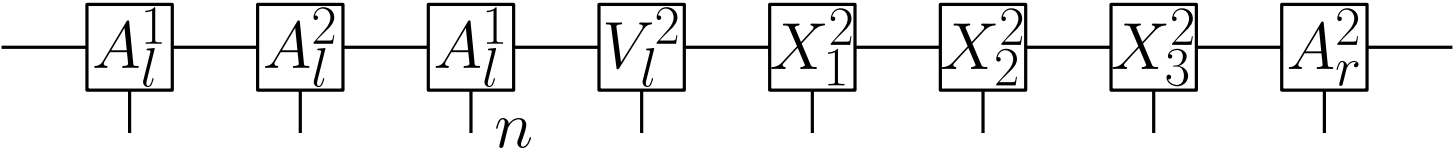

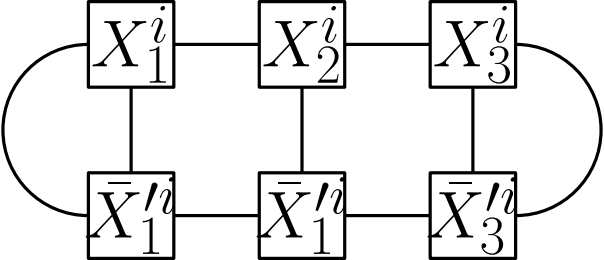

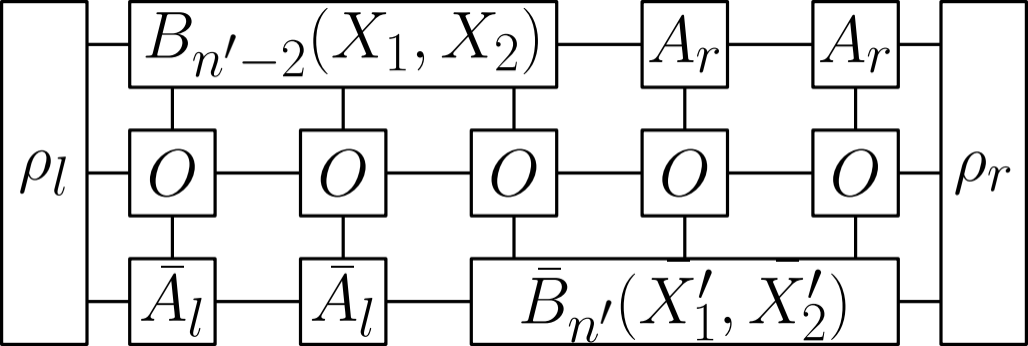

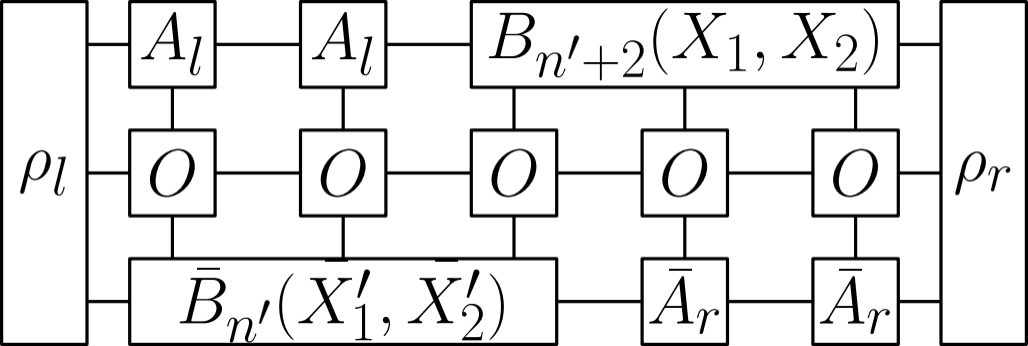

Supplement: Supplementary file 1 [file diagrams_appendix.pdf]
